# Supplementary material for: Z-boson production in p-Pb collisions at $\sqrt{s_{\mathrm{NN}}}=8.16$ TeV and Pb-Pb collisions at $\sqrt{s_{\mathrm{NN}}}=5.02$ TeV
Source: arXiv:2005.11126 source file (2021-03-05)
Supplement: Supplementary file 1 [file appendix.tex]

\section{Numerical values of results}
\label{sex:appendix}

The following tables give the numerical values of the cross section, normalized invariant yield and \Raa presented in the previous sections.

%%%%%%% PROTON LEAD %%%%%%%%%%%%%
\begin{table}[h]
\centering
\begin{tabular}{c|c}
  \hline
  Dimuon rapidity (cms) & $\sigma_{Z \rightarrow \mu^+\mu^-}$, p--Pb, \eightnn \\
  \hline \hline
  $-4.46 < \ycms < -2.96$   & $3.69 \pm 0.65 (\mathrm{stat.}) \pm 0.24 (\mathrm{syst.})$ nb \\
  $2.03 < \ycms < 3.53$     & $10.27\pm 1.29 (\mathrm{stat.})\pm 0.84 (\mathrm{syst.})$ nb \\
  \hline
\end{tabular}
\caption{Values of  $\mathrm{Z} \rightarrow \mu^+\mu^-$ production cross section measured in p-going and Pb-going configurations at \eightnn.}
\label{table:pPbresults}
\end{table}

%%%%%%%%%% LEAD LEAD - YIELD %%%%%%%%%%%%%
\begin{table}[h]
\centering
\begin{tabular}{c|c|c}
  \hline
  Dimuon rapidity  & Centrality class & $\frac{\mathrm{d}N/\mathrm{d}y}{\left< T_{\rm AA} \right>}$, Pb--Pb, \fivenn \\
  \hline \hline
  $2.5<y<4$  &  0-90\%  & $6.13 \pm 0.44 (\mathrm{stat.}) \pm 0.39 (\mathrm{syst.})$ pb \\
  \hline
  $2.5<y<2.8$ &        & $7.24\pm 1.04 (\mathrm{stat.}) \pm 0.46 (\mathrm{syst.})$ pb  \\
  $2.8<y<3.1$ & 0-90\% & $13.24\pm 1.46(\mathrm{stat.}) \pm 0.83 (\mathrm{syst.})$ pb \\
  $3.1<y<4$   &        & $3.33\pm 0.43 (\mathrm{stat.}) \pm 0.21 (\mathrm{syst.})$ pb \\
  \hline
  $2.50 < y < 2.75$ &        &$7.26 \pm 1.15 (\mathrm{stat.}) \pm 0.46 (\mathrm{syst.})$ pb \\
  $2.75 < y < 3.00$ & 0-90\% &$11.37 \pm 1.46 (\mathrm{stat.}) \pm 0.72 (\mathrm{syst.})$ pb \\
  $3.00 < y < 3.25$ &        &$12.05 \pm 1.54 (\mathrm{stat.}) \pm 0.76 (\mathrm{syst.})$ pb \\
  $3.25 < y < 4.00$ &        &$1.99 \pm 0.36 (\mathrm{stat.}) \pm 0.13 (\mathrm{syst.})$ pb \\
  \hline
             & 0-10\%  & $5.29\pm 0.63 (\mathrm{stat.}) \pm 0.33 (\mathrm{syst.})$ pb \\
  $2.5<y<4$  & 10-20\% & $7.26\pm 0.93 (\mathrm{stat.}) \pm 0.46 (\mathrm{syst.})$ pb \\
             & 20-90\% & $6.26\pm 0.75 (\mathrm{stat.}) \pm 0.40 (\mathrm{syst.})$ pb \\
  \hline
\end{tabular}
\caption{Values of the $\mathrm{Z} \rightarrow \mu^+\mu^-$ normalized yield measured in Pb--Pb collisions at \fivenn. The rapidity dependent results are integrated over centrality and vice versa. The quoted systematic is the sum in quadrature of correlated and uncorrelated sources. The correlated systamtics amount to 1.2\% versus rapidity and 6.1\% versus centrality.}
\label{table:PbPbYield}
\end{table}

%%%%%%%%%% LEAD LEAD - RAA %%%%%%%%%%%%%%%
\begin{table}[h]
\centering
\begin{tabular}{c|c|c}
  \hline
  Dimuon rapidity  & Centrality class & $\Raa$, Pb--Pb, \fivenn \\
  \hline \hline
  $2.5<y<4$  &  0-90\%  & $0.770 \pm 0.055 (\mathrm{stat.}) \pm 0.057 (\mathrm{syst.})$ \\
  \hline
  $2.5<y<2.8$ &        & $0.923\pm 0.132 (\mathrm{stat.}) \pm 0.067 (\mathrm{syst.})$   \\
  $2.8<y<3.1$ & 0-90\% & $0.811\pm 0.089(\mathrm{stat.}) \pm 0.059 (\mathrm{syst.})$  \\
  $3.1<y<4$   &        & $0.644\pm 0.083 (\mathrm{stat.}) \pm 0.050 (\mathrm{syst.})$  \\
  \hline
             & 0-10\%  & $0.666\pm 0.079 (\mathrm{stat.}) \pm 0.049 (\mathrm{syst.})$  \\
  $2.5<y<4$  & 10-20\% & $0.914\pm 0.117 (\mathrm{stat.}) \pm 0.067 (\mathrm{syst.})$  \\
             & 20-90\% & $0.787\pm 0.095 (\mathrm{stat.}) \pm 0.059 (\mathrm{syst.})$  \\
  \hline
\end{tabular}
\caption{Values of the Z boson \Raa  measured in Pb--Pb collisions at \fivenn. The rapidity dependent results are integrated over centrality and vice versa. The quoted systematic is the sum in quadrature of correlated and uncorrelated sources. The correlated systamtics amount to 1.2\% versus rapidity and 7.3\% versus centrality; they include the uncertainty on the CT14 NLO~\cite{ct14} proton-proton cross section used as reference.}
\label{table:PbPbRaa}
\end{table}
